# Supplementary material for: From Simulation to Real-World Robotic Mobile Fulfillment Systems
Source: arXiv:1810.03643 source file (2018-10-08)
Supplement: Supplementary file 1 [file appendix.tex]

\appendix

\subsection{Hard to prove}

\global\long\def\DepartureTime{D}

\begin{prop}
Under \assuref{long-term-average-exists} the long term costs can
be calculated
\end{prop}
\begin{align*}
\overline{\dpNstagecosts_{\pi}} & :=\left(\mathbb{E}\left(\frac{1}{N}\sum_{t=0}^{N-1}\sum_{\stationelement\in\stationset}\left(\coststostation(\pi(t),s)\right)\right)+\sum_{\stationelement\in\stationset}\costsfromstation(S(t),\pi(t))\right)
\end{align*}
where $S(t)$ is a sequence of stations from where a shelf departures
at time $t$.
\begin{proof}
Let $P(t)$ be a sequence of places where the shelves departure at
time $t$. 

\begin{equation}
\overline{\dpNstagecosts_{\pi}}:=\lim_{N\rightarrow\infty}\frac{1}{N}\sum_{t=0}^{N-1}\left(\coststostation(P(t),\stationprojection{\randomtask(t)})+\costsfromstation(S(t),\pi(t))\right)\qquad a.s.\label{eq:simplified-convergency-step-1}
\end{equation}

Let $\DepartureTime(t,N)\in[0,N]$ be a function which indicates when
the shelf which was assignet by policy $\pi(t)$ will departure later
from the storage space within time span $[0,N-1]$. $\DepartureTime(t,N):=N$
when the shelf will not departure within $[0,N-1]$ .

\begin{align*}
\frac{1}{N}C_{N\pi} & =\frac{1}{N}\sum_{t=0}^{N-1}\left(\coststostation(P(t),\stationprojection{\randomtask(t)})+\costsfromstation(S(t),\pi(t))\right)\cdot1_{[\DepartureTime(t,N)<N]}\\
 & \hphantom{=}+\frac{1}{N}\underbrace{\sum_{t=0}^{N-1}\left(\coststostation(P(t),\stationprojection{\randomtask(t)})+\costsfromstation(S(t),\pi(t))\right)\cdot1_{[\DepartureTime(t,N)=N]}}_{\text{bounded}}
\end{align*}

The second summand almost surely converges to $0$, because  for every
$\omega\in\Omega$ the indicator $1_{[\DepartureTime(t,N)=N]}(\omega)$
is almost always zero. $1_{[\DepartureTime(t,N)=N]}(\omega)$ cannot
be more more 1 than the maximal number of shelves in the storage.

We focus now on the first summand. For every $\omega\in\Omega$ with
$1_{[\BusyEnd t<N]}=1$ a shelf which was previously assigned by $\pi(\omega;t)$
will leave the storage until time $N$. Thefore first summand converge
to the same value as the sequence

\[
f_{N}:=\frac{1}{N}\sum_{t=0}^{N-1}\left(\coststostation(\pi(t),\stationprojection{\randomtask(\DepartureTime(t,N))})\cdot1_{[\DepartureTime(t,N)<N]}+\costsfromstation(S(t),\pi(t))\right)
\]

The sequence $f_{N}$ is bounded and converges to a constant $C_{N\pi}$
therefore
\[
\mathbb{E}\left(\lim_{N\rightarrow\infty}f_{N}\right)=\lim_{N\rightarrow\infty}\mathbb{E}(f_{N})
\]
 we calculate $\mathbb{E}(f_{N})$
\begin{align*}
\lim_{N\rightarrow\infty}\mathbb{E}(f_{N}) & =\lim_{N\rightarrow\infty}\mathbb{E}\left(\frac{1}{N}\sum_{t=0}^{N-1}\left(\coststostation(\pi(t),\stationprojection{\randomtask(\DepartureTime(t,N))})\cdot1_{[\DepartureTime(t,N)<N]}\right.\right.\\
 & +\left.\vphantom{\frac{1}{N}\sum_{t=0}^{N-1}}\left.\vphantom{\left(\coststostation(\pi(t),\stationprojection{\randomtask(\DepartureTime(t,N))})\cdot\right.}\costsfromstation(S(t),\pi(t))\right)\right)\\
 & =\lim_{N\rightarrow\infty}\Bigg(\mathbb{E}\left(\frac{1}{N}\sum_{t=0}^{N-1}\left(\coststostation(\pi(t),\stationprojection{\randomtask(\DepartureTime(t,N))})\right)\cdot1_{[\DepartureTime(t,N)<N]}\right)\\
 & +\sum_{\stationelement\in\stationset}\costsfromstation(S(t),\pi(t))\Bigg)
\end{align*}

Because the choice of the future station does not depend on $\pi(t)$
weh have
\begin{align*}
 & \lim_{N\rightarrow\infty}\left(\mathbb{E}\left(\frac{1}{N}\sum_{t=0}^{N-1}\sum_{\stationelement\in\stationset}\left(\coststostation(\pi(t),s)\right)\cdot1_{[\DepartureTime(t,N)<N]}\right)+\sum_{\stationelement\in\stationset}\costsfromstation(S(t),\pi(t))\right)
\end{align*}
and following
\[
\left(\mathbb{E}\left(\frac{1}{N}\sum_{t=0}^{N-1}\sum_{\stationelement\in\stationset}\left(\coststostation(\pi(t),s)\right)\right)+\sum_{\stationelement\in\stationset}\costsfromstation(S(t),\pi(t))\right)
\]
\end{proof}
